# Supplementary material for: Canonical Quantization of Crystal Dislocation and Electron-Dislocation Scattering in an Isotropic Medium
Source: arXiv:1512.01856 ancillary file (2016-05-25)
Supplement: Supplementary file 1 [file Supplemental_Materials.pdf]

## Supplemental Materials of "*Canonical Quantization of Crystalline Dislocation and Electron-Dislocation Scattering in an Isotropic Medium*"

Mingda Li, Wenping Cui, Mildred. S. Dresselhaus and Gang Chen

### A. Dislocation's displacement using Green's function method

Defining $\mathbf{u}(\mathbf{R})$ as the displacement at spatial point **R**, the spatial derivative tensor of $\mathbf{u}$, say distortion tensor, can be written as $\omega_{ij} \equiv \partial u_i / \partial R_j$ , from which we define the symmetric strain tensor as [S1]

$$u_{ij} = \frac{1}{2}\left(\omega_{ij} + \omega_{ji}\right) = \frac{1}{2}\left(\frac{\partial u_i}{\partial R_j} + \frac{\partial u_j}{\partial R_i}\right) \tag{A1}$$

The relation between the stress and strain tensor can be found by generalized Hooke's law

$$\sigma_{ij} = c_{ijkl} u_{kl} \tag{A2}$$

In an isotropic medium, the elastic constants tensor is given by

$$c_{ijkl} = \lambda \delta_{ij}\delta_{kl} + \mu(\delta_{ik}\delta_{jl} + \delta_{il}\delta_{jk}) \tag{A3}$$

where $\lambda$ is the Lamé's 1$^{st}$ constant while $\mu$ is the modulus of rigidity (shear modulus).

As equilibrium, the internal stress in each direction must balance with external force, hence the local force equilibrium can be written as

$$f_i = -\frac{\partial \sigma_{ij}}{\partial R_j} = -c_{ijkl}\frac{\partial u_{kl}}{\partial R_j} \tag{A4}$$

where $f_i$ is the body force per unit volume (*i*,*j* = 1,2,3).

Eq. (A4) is a 2$^{nd}$ order linear inhomogeneous differential equation, hence can be solved using Green's function method. Defining Green's function as

$$\delta_{im}\delta^{(3)}(\mathbf{R}-\mathbf{R}') = -c_{ijkl}\frac{\partial^2 G_{km}(\mathbf{R}-\mathbf{R}')}{\partial R_j \partial R_l} \tag{A5}$$

Now we define the Fourier transformed Green's function as $G_{ij}(\mathbf{k}) \equiv \int G_{ij}(\mathbf{R}) e^{-i\mathbf{k}\cdot\mathbf{R}} d^3\mathbf{R}$

In an isotropic media and in momentum space, eq. (A5) can be solved using Fourier transform method as

$$G_{ij}(\mathbf{k}) = \frac{1}{\mu}\left[\frac{\delta_{ij}}{k^2} - \frac{1}{2(1-\nu)}\frac{k_i k_j}{k^4}\right] \quad \text{(A6)}$$

where $\nu \equiv \frac{\lambda}{2(\lambda+\mu)}$ is the Poisson ratio.

Then the solution of the corresponding inhomogeneous equation can be written from Eq. (A5) as

$$u_i(\mathbf{R}) = \int G_{ij}(\mathbf{R}-\mathbf{R}')f_j(\mathbf{R}')d^3\mathbf{R}' = -c_{jklm}\int u_{lm}(\mathbf{R}')\frac{\partial G_{ij}(\mathbf{R}-\mathbf{R}')}{\partial \mathrm{R}_k}d^3\mathbf{R}' \quad \text{(A7)}$$

Assuming a dislocation loop **D** with local tangent vector $\tau$ . Defining $L$ is an arbitrary contour circling the dislocation loop over the surface $\mathbf{S}_{\mathrm{L}}$. Then the Burgers vector (or the definition of dislocation) can be written as **[S2-S4] (Fig. S1)**

$$\oint_L du_i = \oint_L \omega_{ij}dr_j = -b_i \quad \text{(A8)}$$

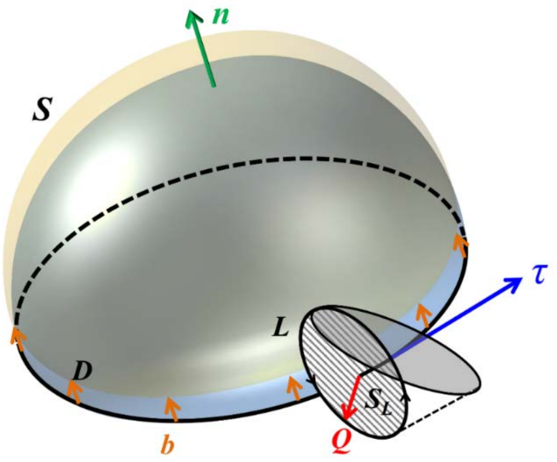


**Fig. S1.** Illustration of a dislocation loop. $L$ is an arbitrary contour circling the dislocation loop over the surface $\mathrm{S}_L$. $Q$ is a 2D position vector along the loop L, which is perpendicular with the tangent vector $\tau$ , hence Q can be understood as the deviation of dislocation away from its original position. Defining $\mathbf{S}_{\mathrm{D}}$ is an arbitrary surface with boundary **D**, which has normal **n** to the dislocation loop, and line element of dislocation is $d\mathbf{l}$.

Now defining the coordinate $\zeta$ which is the coordinate from the surface along the surface normal **n**, then we have $\omega_{ij} = n_i b_j \delta(\zeta)$ on the discontinuity surface, hence

$$u_{lm}(\mathbf{R}') = \frac{1}{2}\left(n_l b_m + n_m b_l\right)\delta\left(\zeta\right) \quad \text{(A9)}$$

The displacement can finally be re-written as [S3]

$$u_i(\mathbf{R}) = -c_{jklm} b_m \oiint_{S_D} n_l \frac{\partial}{\partial R_k} G_{ij}(\mathbf{R}-\mathbf{R}')dS' \qquad \text{(A10)}$$

Assuming that an infinite-long straight dislocation is located at (x,y)=(0,0) along z-direction, with the displacement of the dislocation at position $z$ is $Q(\mathrm{z})$, as shown in the Fig.1 of main text. Then we have

$$u_i(\mathbf{R}) \equiv u_i(\mathbf{r}, z) = -b_m c_{jklm} \int_{-\infty}^{+\infty} n_l \frac{\partial}{\partial R_k} G_{ij}(\mathbf{r}, z-z')Q(z')dz' \qquad \text{(A11)}$$

## B. Expansion of displacement, Kinetic energy and Potential energy

The displacement of dislocation away from straight line can be expanded as [S4]

$$Q(z) = \sum_{\kappa} Q_\kappa e^{i\kappa z} \qquad \text{(B1)}$$

From which we expect the lattice displacement can be expressed as

$$u_i(\mathbf{R}) = \sum_{\kappa} f_i(\mathbf{r} \equiv (x,y);\kappa) e^{i\kappa z} Q_\kappa \qquad \text{(B2)}$$

where $f_i(x,y;\kappa)$ is an expansion coefficient to be determined fro.

Now substitute Eq. (B1) back to Eq. (A11), and comparing with Eq.(B2), we have

$$f_i(\mathbf{r};\kappa) = -b_m c_{jklm} n_l \int_{-\infty}^{+\infty} \frac{\partial}{\partial R_k} G_{ij}(\mathbf{r}, z-z') e^{i\kappa(z'-z)} dz' \qquad \text{(B3)}$$

Defining the 2D Fourier transform of the expansion coefficient the corresponding inverse transform

$$\begin{cases} B_i(\mathbf{s};\kappa) \equiv \int f_i(\mathbf{r} \equiv (x,y);\kappa) e^{-i\mathbf{s}\cdot\mathbf{r}} d^2\mathbf{r} \\ f_i(\mathbf{r} \equiv (x,y);\kappa) = \dfrac{1}{A} \sum_{\mathbf{s}} B_i(\mathbf{s};\kappa) e^{+i\mathbf{s}\cdot\mathbf{r}} \end{cases} \qquad \text{(B4)}$$

which satisfies

$$u_i(\mathbf{R} \equiv (\mathbf{r}, z) = (x,y,z)) = \frac{1}{A} \sum_{\mathbf{s},\kappa} B_i(\mathbf{s};\kappa) e^{+i\mathbf{s}\cdot\mathbf{r}} e^{i\kappa z} Q_\kappa \equiv \frac{1}{A} \sum_{\mathbf{k} \equiv (\mathbf{s},\kappa)} B_i(\mathbf{k}) e^{i\mathbf{k}\cdot\mathbf{R}} Q_\kappa \qquad \text{(B5)}$$

Comparing Eqs. (A6), (A11) and (B5), we finally obtain

$$B_i(\mathrm{s};\kappa) = +\frac{i}{k^2}\left( n_i(\mathbf{b}\cdot\mathbf{k}) + b_i(\mathbf{n}\cdot\mathbf{k}) - \frac{1}{(1-\nu)} \frac{k_i(\mathbf{n}\cdot\mathbf{k})(\mathbf{b}\cdot\mathbf{k})}{k^2} \right) \qquad \text{(B6)}$$

Now we turn to the energy computation. The total kinetic energy of the solid can be written using Eq.  as

$$T = \frac{\rho}{2}\int \sum_{i=1}^{3} \dot{u}_i^2(r)dV \equiv \frac{L}{2}\sum_{\kappa} m(\kappa)\dot{Q}_\kappa \dot{Q}_\kappa^* \qquad \text{(B7)}$$

where

$$\begin{aligned} m(\kappa) &\equiv \frac{\rho}{A}\sum_{i=1}^{3}\sum_{\mathbf{s}} \left|B_i(\mathbf{s};\kappa)\right|^2 \\ &= \frac{\rho}{4\pi^2}\int d^2\mathbf{s} \frac{1}{k^4}\left[ \left(\mathbf{b}\cdot\mathbf{k}\right)^2 + b^2\left(\mathbf{n}\cdot\mathbf{k}\right)^2 + \frac{4\nu-3}{(1-\nu)^2}\frac{\left(\mathbf{n}\cdot\mathbf{k}\right)^2\left(\mathbf{b}\cdot\mathbf{k}\right)^2}{k^2}\right] \end{aligned} \qquad \text{(B8)}$$

which has the linear mass density unit in an effective model, and **s** is the summation of 2D in-plane momentum.

Similarly, total potential energy can be computed  as

$$U = \frac{1}{2}\int \sigma_{ij}u_{ij}d^3\mathbf{R} = \frac{1}{2}\int c_{ijkl}u_{ij}u_{kl}d^3\mathbf{R} = U(\kappa) + U_0 = \frac{L}{2}\sum_{\kappa}\kappa^2 T(\kappa)Q_\kappa Q_\kappa^* \qquad \text{(B9)}$$

where

$$\kappa^2 K(\kappa) \equiv \frac{\mu}{4\pi^2}\int d^2\mathbf{s}\left( \frac{\left(\mathbf{b}\cdot\mathbf{k}\right)^2 + b^2\left(\mathbf{n}\cdot\mathbf{k}\right)^2}{k^2} - \frac{2}{1-\nu}\frac{\left(\mathbf{n}\cdot\mathbf{k}\right)^2\left(\mathbf{b}\cdot\mathbf{k}\right)^2}{k^4}\right) \qquad \text{(B10)}$$

Then we could recover the results from [S4]. The total classical Hamiltonian can be written as

$$H_D = \frac{L}{2}\sum_{\kappa}\left[ m(\kappa)\dot{Q}_\kappa\dot{Q}_\kappa^* + \kappa^2 K(\kappa)Q_\kappa Q^*{}_\kappa \right] \qquad \text{(B11)}$$

For an edge dislocation, we have

$$m_E(\kappa) = \frac{\rho b^2}{4\pi}\left[ \log\left(1+\frac{k_D^2}{\kappa^2}\right) - \frac{k_D^2}{k_D^2+\kappa^2} + \frac{4\nu-3}{8(1-\nu)^2}\left( \log\left(1+\frac{k_D^2}{\kappa^2}\right) - \frac{k_D^2\left(3k_D^2+2\kappa^2\right)}{2\left(k_D^2+\kappa^2\right)^2}\right)\right]$$

$$K_E(\kappa) = \frac{\mu b_x^2}{4\pi}\left[ \frac{1-2\nu}{2(1-\nu)}\log\frac{k_D^2}{\kappa^2} + 1 - \frac{1}{4(1-\nu)}\frac{\kappa^2}{k_D^2}\right]$$

For a screw dislocation, we have

$$m_S(\kappa)=\frac{\rho b^2}{4\pi}\left[\frac{k_D^2}{2(\kappa^2+k_D^2)}+\frac{1}{2}\log\left(1+\frac{k_D^2}{\kappa^2}\right)+\frac{4\nu-3}{4(1-\nu)^2}\frac{k_D^4}{\left(k_D^2+\kappa^2\right)^2}\right]$$

$$K_S(\kappa)=\frac{\mu b_z^2}{4\pi}\left[\frac{1+\nu}{2(1-\nu)}\left(\log\frac{k_D^2}{\kappa^2}-1\right)+\frac{1}{1-\nu}\frac{\kappa^2}{k_D^2}\right]$$

## C. Canonical Quantization of Dislocation

We **impose** the canonical quantization condition

$$Q_\kappa = Z_{\mathrm{k}}(a_\kappa + a_{-\kappa}^+) \tag{C1}$$

Satisfying the commutation relation

$$[Q_\kappa, P_{\kappa'}] = i\hbar\delta_{\kappa,\kappa'} \tag{C2}$$

Then the following pair of operator

$$\begin{cases} Q_\kappa = Z_\kappa\left[a_\kappa + a_{-\kappa}^+\right] \\ P_\kappa = \dfrac{i\hbar}{2Z_\kappa}\left[a_\kappa^+ - a_{-\kappa}\right] \end{cases} \tag{C3}$$

will satisfy both canonical relation $[a_\kappa, a_{\kappa'}^+] = \delta_{\kappa,\kappa'}$ and Eq. (C3), simultaneously.

On the other hand, the conjugate momentum $P_\kappa = \frac{\partial\mathcal{L}}{\partial\dot{Q}_\kappa} = Lm(\kappa)\dot{Q}_\kappa^*$, which gives $Z_\kappa = \sqrt{\frac{\hbar}{2Lm(\kappa)\omega(\kappa)}}$. Hamiltonian of dislocation Eq. (B11) can finally be written as

$$H_D = \sum_\kappa \hbar\omega(\kappa)\left[a_\kappa^+ a_\kappa + \frac{1}{2}\right] \tag{C4}$$

where the eigen-frequency $\omega(\kappa) \equiv \kappa\sqrt{\frac{K(\kappa)}{m(\kappa)}}$. For an edge dislocation, the quantized eigen-frequency gives

$$\omega_E(\kappa) = v_s\kappa\sqrt{\frac{\frac{1-2\nu}{2(1-\nu)}\log\left(\frac{k_D^2}{\kappa^2}+1\right)+1-\frac{1}{4(1-\nu)}\frac{\kappa^2}{k_D^2+\kappa^2}}{\log\left(1+\frac{k_D^2}{\kappa^2}\right)-\frac{k_D^2}{k_D^2+\kappa^2}+\frac{4\nu-3}{8(1-\nu)^2}\left(\log\left(1+\frac{k_D^2}{\kappa^2}\right)-\frac{k_D^2\left(3k_D^2+2\kappa^2\right)}{2\left(k_D^2+\kappa^2\right)^2}\right)}}$$

While for a screw dislocation, the quantized eigen-frequency gives

$$\omega_S(\kappa) = v_s\kappa\sqrt{\frac{\frac{1+\nu}{2(1-\nu)}\left(\log\left(1+\frac{k_D^2}{\kappa^2}\right)-1\right)+\frac{1}{1-\nu}\frac{\kappa^2}{k_D^2+\kappa^2}}{\frac{k_D^2}{2(\kappa^2+k_D^2)}+\frac{1}{2}\log\left(1+\frac{k_D^2}{\kappa^2}\right)+\frac{4\nu-3}{4(1-\nu)^2}\frac{k_D^4}{\left(k_D^2+\kappa^2\right)^2}}}$$

## D. Hamiltonian of electron-dislocation interaction

We start from a lattice model, that $\mathbf{R}_j = \mathbf{R}_j^0 + \mathbf{u}_j$, and there are N sites of the system. Assuming the electron charge density is $\rho_e(\mathbf{R})$, the electron-ion interaction Hamiltonian can be written as [S5],

$$\begin{aligned} H_{\text{int}} &= \int d^3\mathbf{R}\rho_e(\mathbf{R})\sum_{j=1}^{N}V_{ei}(\mathbf{R}-\mathbf{R}_j) \\ &\simeq \int d^3\mathbf{R}\rho_e(\mathbf{R})\sum_{j=1}^{N}V_{ei}(\mathbf{R}-\mathbf{R}_j^0) + \int d^3\mathbf{R}\rho_e(\mathbf{R})\sum_{j=1}^{N}\nabla_{\mathbf{R}}V_{ei}(\mathbf{R}-\mathbf{R}_j^0)\cdot\mathbf{u}_j \end{aligned} \tag{D1}$$

where the 1st term gives the ion potential function which electrons travel within the periodic potential of a crystal, i.e. Bloch waves, and the 2nd term gives both electron-phonon and electron-dislocation scattering.

To further simplify Eq. (D1), we note that the electron charge density can be written in terms of number density as

$$\rho_e(\mathbf{R}) = en_e(\mathbf{R}) = \frac{e}{V}\sum_{\mathbf{kp}\sigma}e^{+i\mathbf{p}\cdot\mathbf{R}}c_{\mathbf{k}+\mathbf{p}\sigma}^{+}c_{\mathbf{k}\sigma} \tag{D2}$$

While the ionic potential can be expanded as Fourier components

$$\sum_{j=1}^{N}\nabla_{\mathbf{R}}V_{ei}(\mathbf{R}-\mathbf{R}_j^0)\cdot\mathbf{u}_j = \frac{i}{V}\sum_{\mathbf{q}\in 1\text{BZ},\mathbf{G}}V_{\mathbf{q}+\mathbf{G}}e^{i(\mathbf{q}+\mathbf{G})\cdot\mathbf{R}}(\mathbf{q}+\mathbf{G})\cdot\sum_{j=1}^{N}e^{-i(\mathbf{q}+\mathbf{G})\cdot\mathbf{R}_j^0}\mathbf{u}_j \tag{D3}$$

where the screened Coulomb potential $V_{\mathbf{q}} = \frac{4\pi Ze}{q^2 + k_{TF}^2}$.

Substituting Eq. (B5) back to Eq. (D3), and only considering normal process (G=0) instead of Umklapp process, which is suitable for low temperature since phase space for Umklapp process is small, and considering single mode phonon, i.e. isotropic case for normal dislon mode (Jellium model), Eq. (D3) can finally be simplified as

$$\begin{aligned}&\sum_{j=1}^{N} \nabla_{\mathbf{R}} V_{ei}(\mathbf{R} - \mathbf{R}_j^0) \cdot \mathbf{u}_j \\ &= -\frac{N}{V} \sum_{\mathbf{q}} V_{\mathbf{q}} e^{i\mathbf{q}\cdot\mathbf{R}} \frac{1-2\nu}{1-\nu} \frac{(\mathbf{b}\cdot\mathbf{q})(\mathbf{n}\cdot\mathbf{q})}{q^2} \frac{1}{A} \sqrt{\frac{\hbar}{2Lm(\kappa)\omega(\kappa)}} \left(a_\kappa + a_{-\kappa}^+\right)\end{aligned} \tag{D4}$$

where we have used the fact that $\sum_{j=1}^{N} e^{+i(\mathbf{k}-\mathbf{q}-\mathbf{G})\cdot\mathbf{R}_j^0} = N\delta_{\mathbf{k},\mathbf{q}+\mathbf{G}}$ valid.

This gives an important prediction: in the isotropic upper limit $\nu = 1/2$, there is no electron-dislocation scattering. This is quite reasonable, since at this limit, the stiffness decreases greatly (Young's modulus E=0, and shear modulus G=0) like a rubber (which has $\nu = 1/2$), in which case the deformation is fully elastic but dislocation is plastic, i.e. cannot emerge.

In this situation, the electron-dislocation scattering Hamiltonian can finally be written as

$$\begin{aligned}&H_{e-dis} = -\frac{Ne^2}{V}\frac{1-2\nu}{1-\nu} \times \\ &\sum_{\kappa} \sqrt{\frac{\hbar}{2Lm(\kappa)\omega(\kappa)}} \iint \frac{sdsd\theta}{\pi} \frac{(b_x s\cos\theta + b_z\kappa) s\sin\theta}{(s^2+\kappa^2+k_{TF}^2)(s^2+\kappa^2)} \rho(\mathbf{s};\kappa)\left(a_\kappa + a_{-\kappa}^+\right)\end{aligned} \tag{D5}$$

For a single electron located at $\mathbf{R} = (\mathbf{r}, z) = (r\cos\phi, r\sin\phi, z)$, we have $\rho(\mathbf{s};\kappa) = \exp\left(i\mathbf{s}\cdot\mathbf{r} + i\kappa z\right)$, hence the Hamiltonian Eq. (D5) can be re-written as

$$H_{e-dis} = \frac{1}{\sqrt{L}} \sum_{\kappa} e^{i\kappa z} M_{\mathbf{b},\mathbf{r}}(\kappa)\left(a_\kappa + a_{-\kappa}^+\right) \tag{D6}$$

with coupling constant defined as

$$M_{\mathbf{b},\mathbf{r}}(\kappa) \equiv \frac{Ne^2}{V}\frac{1-2\nu}{1-\nu}\sqrt{\frac{\hbar}{2m(\kappa)\omega(\kappa)}} \int s^2 ds \frac{b_x s J_2(rs)\sin 2\phi - 2ib_z\kappa J_1(rs)\sin\phi}{(s^2+\kappa^2+k_{TF}^2)(s^2+\kappa^2)}$$

Using the asymptotic form $J_n(z) \xrightarrow{z\to\infty} \sqrt{\frac{2}{\pi z}} \cos\left(z - \frac{n\pi}{2} - \frac{\pi}{4}\right)$. We have

$$M_{\mathbf{b},\mathbf{r}}(\kappa) \equiv + \frac{Ne^2}{V} \frac{1-2\nu}{1-\nu} \sqrt{\frac{2}{\pi r}} \sqrt{\frac{\hbar}{2m(\kappa)\omega(\kappa)}} \times$$
$$\int ds \frac{b_x s^{5/2} \cos(rs - \frac{5\pi}{4}) \sin 2\phi - 2ib_z \kappa s^{+3/2} \cos(rs - \frac{3\pi}{4}) \sin\phi}{(s^2+\kappa^2+k_{TF}^2)(s^2+\kappa^2)} \tag{D7}$$

Now we assume that the Coulomb screening is weak ( $k_{TF} = 0$ ), and simplify the integration range $s \in [0, k_D] \to [0, +\infty]$ , we have

$$M_{\mathbf{b},\mathbf{r}\to\infty}(\kappa) = + \frac{Ne^2}{8V} \frac{1-2\nu}{1-\nu} \sqrt{\frac{\hbar\pi}{m(\kappa)\omega(\kappa)\kappa r}} \times$$
$$\left[ b_x (2\kappa r - 3) \sin 2\phi - 2ib_z (2\kappa r - 1) \sin\phi \right] \exp(-\kappa r) \tag{D8}$$

Therefore, we have

$$\left| M_{\substack{edge \\ \mathbf{r}\to\infty}}(\kappa) \right|^2 = \left( \frac{Ne^2}{8V} \right)^2 \left( \frac{1-2\nu}{1-\nu} \right)^2 \frac{\hbar\pi b^2 (2\kappa r - 3)^2}{m(\kappa)\omega(\kappa)\kappa r} \sin^2 2\phi \exp(-2\kappa r)$$
$$\left| M_{\substack{screw \\ \mathbf{r}\to\infty}}(\kappa) \right|^2 = + \left( \frac{Ne^2}{8V} \right)^2 \left( \frac{1-2\nu}{1-\nu} \right)^2 \frac{4\hbar\pi b^2 (2\kappa r - 1)^2}{m(\kappa)\omega(\kappa)\kappa r} \sin^2 \phi \exp(-2\kappa r) \tag{D9}$$

for edge and screw dislocation, respectively.

## E. Feynman rules of quantized electron-dislocation interaction

We can write down the **Feynman Rules** for dislon-electron scattering:

1) Each internal electron line gives $G^{(0)}(\mathbf{p}, ip_n)$ , $p_n = \frac{(2n+1)\pi}{\beta}$
2) Each internal dislocation line gives $\left| M_{\mathbf{b},\mathbf{r}}(\kappa) \right|^2 D^{(0)}(\kappa, i\omega_m)$ , $\omega_m = \frac{2m\pi}{\beta}$ , where

   $D^{(0)}(\kappa, i\omega_n) = -\frac{2\omega_\kappa}{\omega_n^2 + \omega_\kappa^2}$ .
3) Sum over all internal degrees of freedom under the constraint of momentum and frequency conservation.

4) Multiply the expression by $\frac{(-1)^{K+F}(2S+1)^{F}}{(\beta L)^{K}}$, where F is the number of closed Fermion loops, K is the diagram order: for electron self-energy, K is the number of internal phonon lines, for dislon self-energy, K is the half number of vertices.

In this regard, the first-order electron self-energy can be computed as (Fig. S2)

$$\begin{aligned}\Sigma^{(1)}(\mathbf{r},\mathbf{p},ip_n) &= -\frac{1}{\beta L}\sum_{\kappa,\omega_m}\left|M_{\mathbf{b},\mathbf{r}}(\kappa)\right|^2 D^{(0)}(\kappa,i\omega_m)G^{(0)}(\mathbf{p}+\kappa,ip_n+i\omega_m)\\ &= \frac{1}{L}\sum_{\kappa}\left|M_{\mathbf{b},\mathbf{r}}(\kappa)\right|^2\left[\frac{n_B(\omega_\kappa)+n_F(\varepsilon_{\mathbf{p}+\kappa})}{ip_n-\varepsilon_{\mathbf{p}+\kappa}+\omega_\kappa}+\frac{n_B(\omega_\kappa)+1-n_F(\varepsilon_{\mathbf{p}+\kappa})}{ip_n-\varepsilon_{\mathbf{p}+\kappa}-\omega_\kappa}\right]\end{aligned} \tag{E1}$$

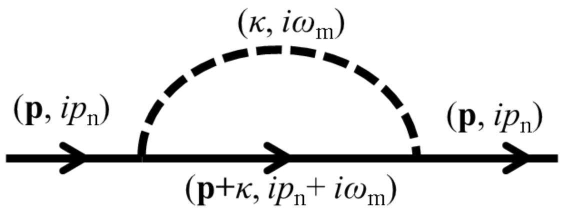


**Fig. S2.** First-order loop correction of electron-quantized dislocation interaction.

Now we assume at $T$=0, where there is only spontaneous emitted dislon without any thermally excited dislon occupancy, $n_B(\omega_\kappa)=0$ and $n_F(\varepsilon_{\mathbf{p}+\kappa})=0$, the self-energy can be written as

$$\Sigma_{RS}^{(1)}(\mathbf{r},\mathbf{p}) = \int\frac{d\kappa}{2\pi}\frac{\left|M_{\mathbf{b},\mathbf{r}}(\kappa)\right|^2}{\varepsilon_{\mathbf{p}}-\varepsilon_{\mathbf{p}+\kappa}-\omega_\kappa+i\delta} \tag{E2}$$

## E. Dimensions of all factors appearing in the calculation

$[Q_\kappa]=\mathrm{L}^{+1}$, $[Q(z)]=\mathrm{L}^{+1}$, $[f_i(x,y;\kappa)]=\mathbf{1}$, $[\mathbf{u}(\mathrm{R}_\mathrm{i}^0)]=\mathrm{L}^{+1}$, $[B_i(\mathrm{s};\kappa)]=\mathrm{L}^{+2}$, $[m(\kappa)]=\mathrm{M}^{+1}\mathrm{L}^{-1}$, $[T]=\mathrm{M}^{+1}\mathrm{L}^{2}\mathrm{T}^{-2}$, $[\mu]=\mathrm{M}^{1}\mathrm{L}^{-1}\mathrm{T}^{-2}$, $[K(\kappa)]=\mathrm{M}^{+1}\mathrm{L}^{+1}\mathrm{T}^{-2}$, $[V]=\mathrm{M}^{+1}\mathrm{L}^{2}\mathrm{T}^{-2}$. $[Z_k]=\mathrm{L}$, $[\mathrm{P}(\kappa)]=\mathrm{M}^{+1}\mathrm{L}^{+1}\mathrm{T}^{-1}$, $[\hbar]=\mathrm{M}^{+1}\mathrm{L}^{+2}\mathrm{T}^{-1}$, $[\omega(\kappa)]=\mathrm{T}^{-1}$, $[\sqrt{\hbar/m(\kappa)/\omega(\kappa)}]=\mathrm{L}^{+3/2}$. $[e]=\mathrm{M}^{1/2}\mathrm{L}^{3/2}\mathrm{T}^{-1}$ (**Static Coulomb**), $[\rho_e(\mathrm{r})]=\mathrm{M}^{1/2}\mathrm{L}^{-3/2}\mathrm{T}^{-1}$, $[V_\mathrm{q}]=\mathrm{M}^{+1/2}\mathrm{L}^{+7/2}\mathrm{T}^{-1}$, $[V_{ei}(\mathrm{r})]=\mathrm{M}^{+1/2}\mathrm{L}^{+1/2}\mathrm{T}^{-1}$. $[\sqrt{\hbar/m(\kappa)/\omega(\kappa)}]=\mathrm{L}^{+3/2}$, $[\rho(\mathbf{q})]=1$, $[H]=\mathrm{M}^{+1}\mathrm{L}^{2}\mathrm{T}^{-2}$, $[M_{\mathbf{b},\mathbf{r}}(\kappa)]=\mathrm{M}^{+1}\mathrm{L}^{+5/2}\mathrm{T}^{-2}$, $[\Sigma_{RS}^{(1)}(\mathbf{r},\mathbf{p})]=\mathrm{M}^{+1}\mathrm{L}^{2}\mathrm{T}^{-2}$.

## References

[S1] E. M. Lifshitz, A. M. Kosevich, and L. P. Pitaevskii, in *Theory of Elasticity (Third Edition)*, edited by E. M. Lifshitz, A. M. Kosevich, and L. P. Pitaevskii (Butterworth-Heinemann, Oxford, 1986), pp. 108.
[S2] F. R. N. Nabarro, *Theory of crystal dislocations* (Oxford, Clarendon P., 1967., 1967), International series of monographs on physics.
[S3] R. Dewit, Solid State Phys **10**, 249 (1960).
[S4] T. Ninomiya, J Res Nbs a Phys Ch **A 73**, 544 (1969).
[S5] G. D. Mahan, *Many-particle physics* (New York : Kluwer Academic/Plenum Publishers, c2000.3rd ed., 2000), Physics of solids and liquids.
